# Supplementary material for: KALA: Knowledge-Augmented Language Model Adaptation
Source: arXiv:2204.10555 source file (2022-08-04)
Supplement: Supplementary file 1 [file casestudy_appendix.tex]

\begin{figure*}[t!]
    \begin{minipage}{0.42\linewidth}
        \centering
        \resizebox{\linewidth}{!}{
            \begin{tabular}{lccl}
            \toprule
            \makecell[l]{Context:
                    A \BLUE{nonsense mutation} in \\
                    \BLUE{exon} 17 ( \BLUE{codon} 556 ) of the RB1 \\
                    \BLUE{gene} was found to be present \\
                    homozygously in both the \RED{retinal} \\ 
                    and the pineal tumours.
            } \\
            \midrule
            Fact: retinal, instance of, gene \\
            \bottomrule
            \end{tabular}
        }
    \end{minipage}
    \begin{minipage}{0.28\linewidth}
        \centering
        \includegraphics[width=1\linewidth]{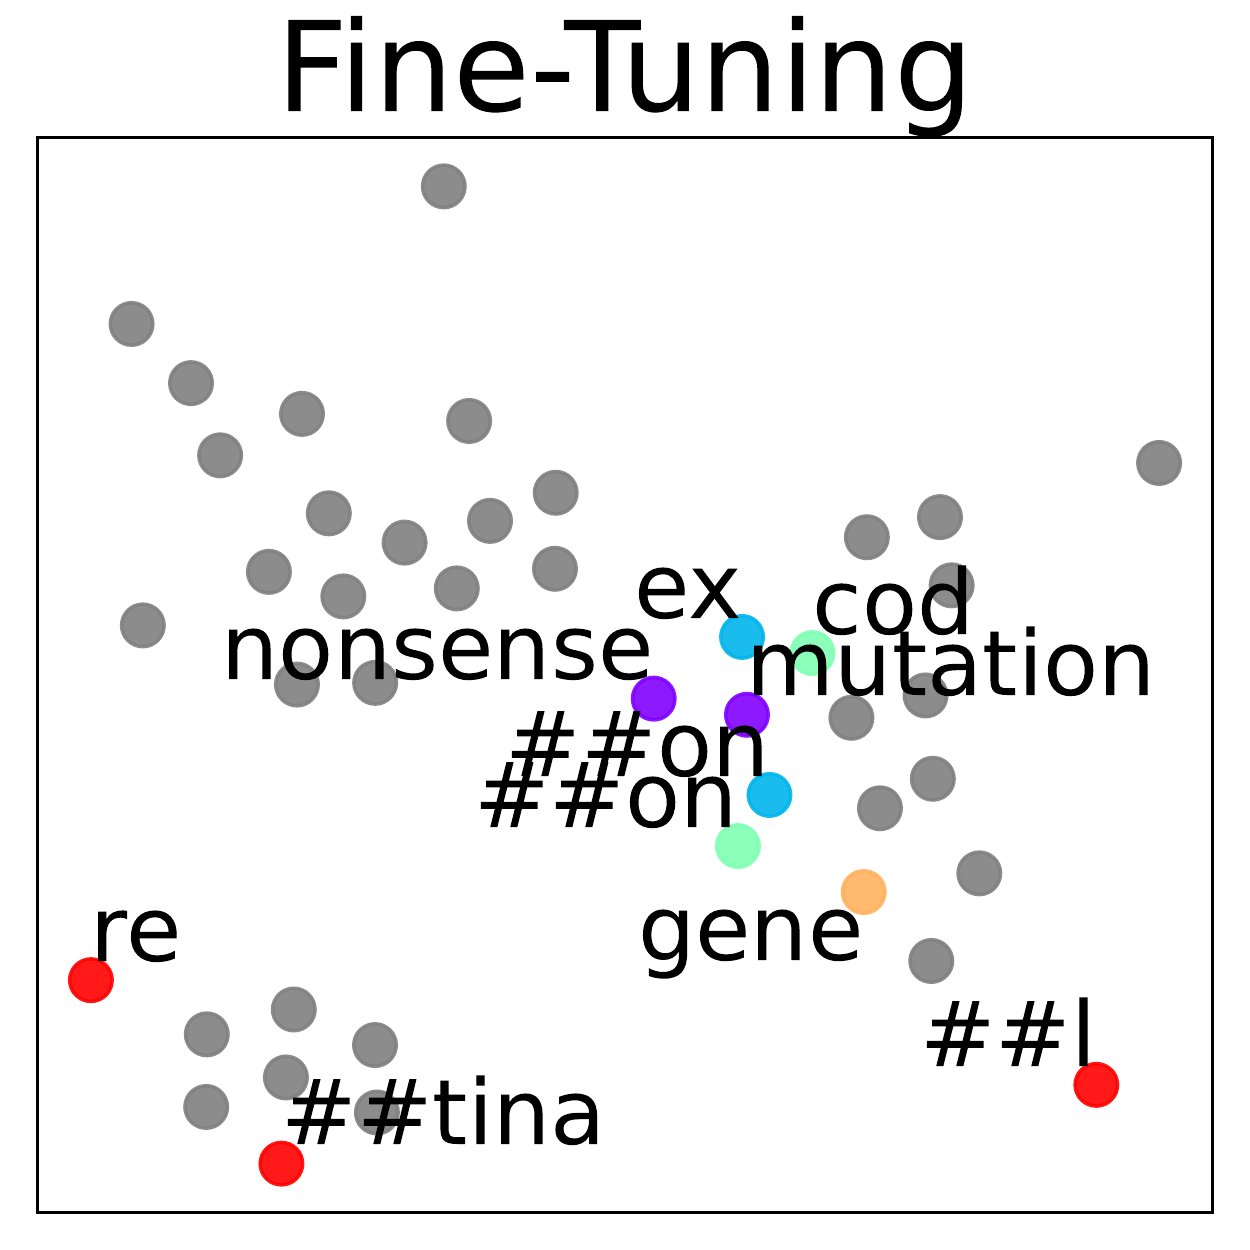}
    \end{minipage}
    \begin{minipage}{0.28\linewidth}
        \centering
        \includegraphics[width=1\linewidth]{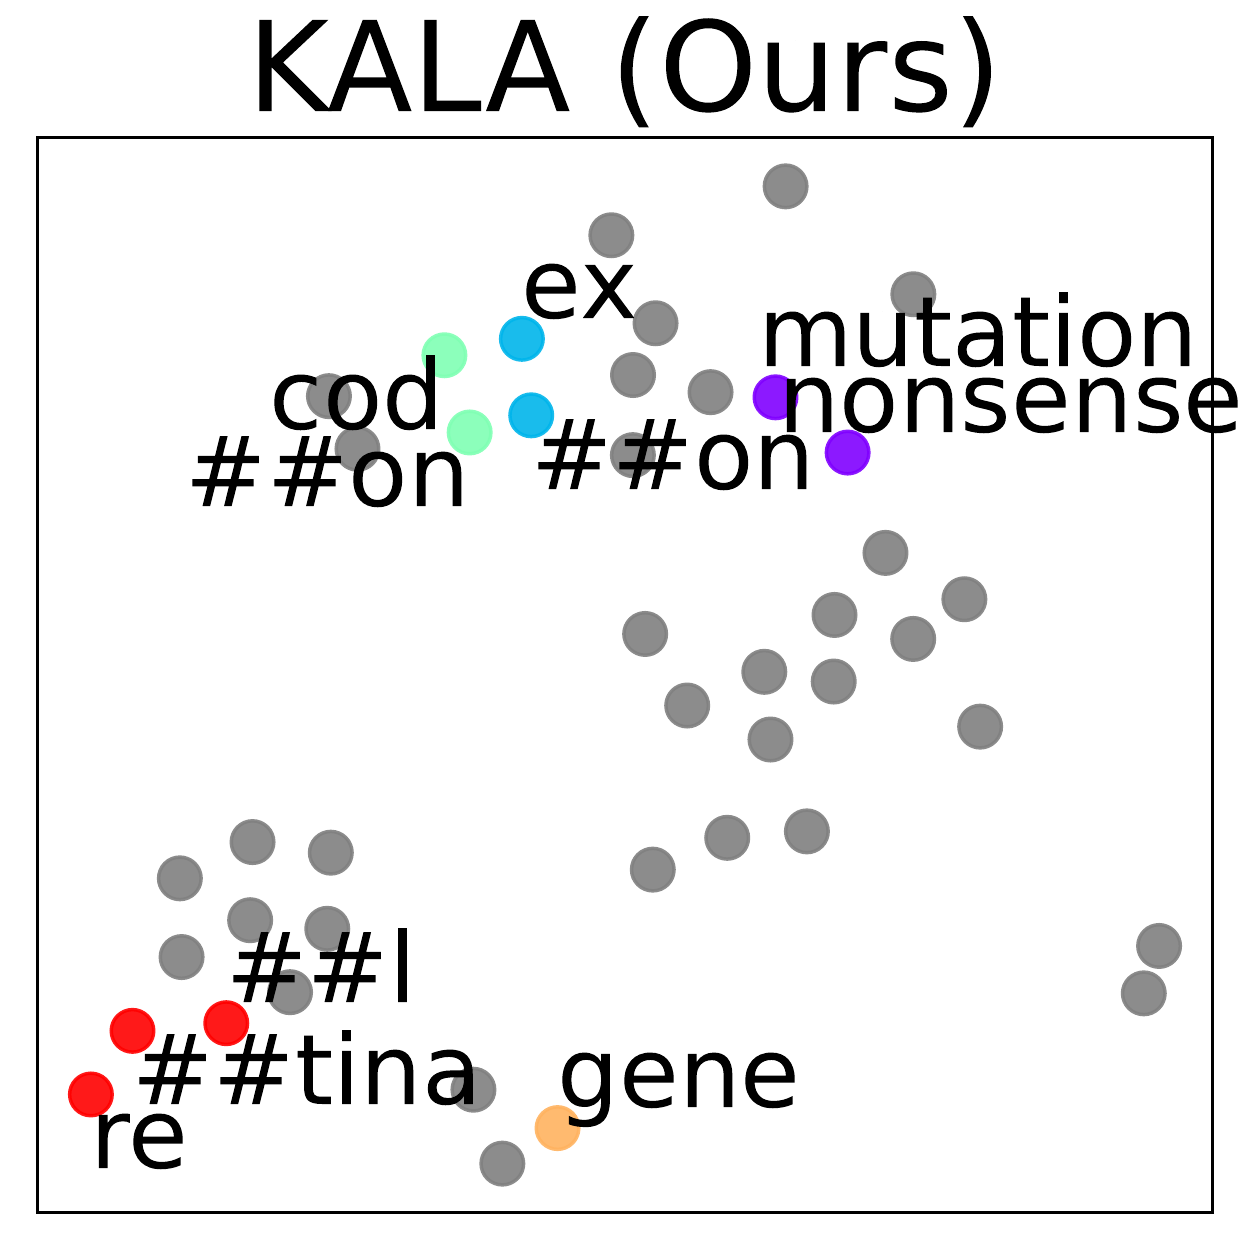}
    \end{minipage}
    \vspace{-0.15in}
    \caption{\small A large version of Figure~\ref{fig:casestudy}}
    \label{fig:casestudy_appendix}
\end{figure*}
