# Supplementary material for: KALA: Knowledge-Augmented Language Model Adaptation
Source: arXiv:2204.10555 source file (2022-08-04)
Supplement: Supplementary file 2 [file miscellaneous.tex]

% \begin{table}[ht]
% \centering
% \resizebox{0.475\textwidth}{!}{
%     \begin{tabular}{lcccccc}
%     \toprule
%     Hyperparameters             & \multicolumn{2}{c}{NewsQA} & \multicolumn{2}{c}{Medication} 
%                                 & \multicolumn{2}{c}{Relation}  \\ 
%                          & BERT & RoBERTa & BERT & RoBERTa & BERT & RoBERTa \\
%     \midrule
%     Learning rate               & \multicolumn{6}{c}{3e-5} \\
%     Batch Size                  & \multicolumn{6}{c}{12} \\
%     Max Sequence                & \multicolumn{6}{c}{384} \\
%     Training Epochs             & \multicolumn{6}{c}{2}    \\
%     \bottomrule
%     \end{tabular}
% }
% \vspace{-0.1in}
% \caption{\small \textbf{Fine-tuning hyperparamters for extractive QA tasks} on three different domain-specific datasets. Max sequence denotes the maximum sequence length of each context.}
% \label{table:hyper-qa}
% \end{table}


% \begin{table}[!t]
% \centering
% \resizebox{0.475\textwidth}{!}{
%     \begin{tabular}{lcccccccc}
%     \toprule
%     Hyperparameters             & \multicolumn{2}{c}{CoNLL-2003} & \multicolumn{2}{c}{WNUT-17} 
%                                 & \multicolumn{2}{c}{NCBI-Disease} \\ 
%                          & BERT & ELECTRA & BERT & ELECTRA & BERT & ELECTRA \\
%     \midrule
%     Learning rate               & \multicolumn{6}{c}{5e-5} \\
%     Batch Size                  & \multicolumn{6}{c}{8} \\
%     Max sequence            & \multicolumn{6}{c}{128} \\
%     Training Epochs             & \multicolumn{6}{c}{5}         \\
%     \bottomrule
%     \end{tabular}
% }
% \vspace{-0.1in}
% \caption{\small \textbf{Fine-tuning Hyperparamters for NER tasks} on three datasets. Max sequence denotes the maximum sequence length of each context.}
% \label{table:hyper-ner}
% \end{table}


% \begin{table*}[t]
% \small
% \centering
% \caption{\small Examples of the OOG link prediction on NELL-995. S: seen, U: unseen, O: correct prediction, X: incorrect prediction, (H): head entity, (R): relation, (T): tail entity, and $\rule{0.2cm}{0.15mm}$: unseen entity.}
% \begin{tabular}{lccl}
% \toprule
% {\bf Type} & {\bf I-GEN} & {\bf T-GEN} & {\bf Triplet}\\
% \midrule
% S-U & O & O & \pbox{50cm}{(H) \underline{musician\_vivaldi}, \\(R) musician\_plays\_instrument, \\(T) music\_instrument\_string} \\
% \midrule
% S-U & O & O & \pbox{50cm}{(H) \underline{city\_hawthorne}, \\(R) city\_located\_in\_state, \\(T) state\_or\_province\_california} \\
% \midrule
% S-U & O & O & \pbox{50cm}{(H) \underline{journalist\_maureen\_dowd}, \\(R) works\_for, \\(T) company\_york\_times} \\
% \midrule
% S-U & O & O & \pbox{50cm}{(H) \underline{person\_monroe}, \\(R) person\_born\_in\_location, \\(T) county\_york\_city} \\
% \midrule
% S-U & O & O & \pbox{50cm}{(H) ceo\_stan\_o\_neal, \\(R) works\_for, \\(T) \underline{retailstore\_merrill}} \\
% \midrule
% S-U & O & O & \pbox{50cm}{(H) insect\_insects, \\(R) invertebrate\_feed\_on\_food
% , \\(T) \underline{agricultural\_product\_wood}} \\
% \midrule
% U-U & X & O & \pbox{50cm}{(H) \underline{person\_katsuaki\_watanabe}, \\(R) person\_leads\_organization, \\(T) \underline{automobilemaker\_toyota}} \\
% \midrule
% U-U & X & O & \pbox{50cm}{(H) \underline{mlauthor\_web\_search}, \\(R) agent\_competes\_with\_agent, \\(T) \underline{website\_altavista\_com}} \\
% \midrule
% U-U & X & O & \pbox{50cm}{(H) \underline{chemical\_chromium}, \\(R) chemical\_is\_type\_of\_chemical, \\(T) \underline{chemical\_heavy\_metals}} \\
% \midrule
% U-U & X & X & \pbox{50cm}{(H) \underline{food\_meals}, \\(R) food\_decreases\_the\_risk\_of\_disease, \\(T) \underline{disease\_heart\_disease}} \\
% \bottomrule
% \end{tabular}
% \label{table:case_study}
% \end{table*}
